# Supplementary material for: Magnetic phases of skyrmion-hosting GaV$_4$S$_{8-y}$Se$_{y}$ ($y = 0, 2, 4, 8$) probed with muon spectroscopy
Source: arXiv:1806.00412 ancillary file (2018-09-11)
Supplement: Supplementary file 1 [file SI.pdf]

# Supplemental Information for "Magnetic phases of skyrmion-hosting $GaV_4S_{8-y}Se_y$ ($y = 0, 2, 4, 8$) probed with muon spectroscopy"

Kévin J. A. Franke,[1] Benjamin M. Huddart,[1] Thomas J. Hicken,[1] Fan Xiao,[2,3] Stephen J. Blundell,[4] Francis L. Pratt,[5] Marta Crisanti,[6,7] Joel A. T. Barker,[8] Stewart J. Clark,[1] Aleš Štefančič,[6] Monica Ciomaga Hatnean,[6] Geetha Balakrishnan,[6] and Tom Lancaster[1]

[1]*Durham University, Centre for Materials Physics, Durham, DH1 3LE, United Kingdom*
[2]*Laboratory for Neutron Scattering, Paul Scherrer Institut, CH-5232 Villigen PSI, Switzerland*
[3]*Department of Chemistry and Biochemistry, University of Bern, CH-3012 Bern, Switzerland*
[4]*Oxford University Department of Physics, Clarendon Laboratory, Parks Road, Oxford OX1 3PU, United Kingdom*
[5]*ISIS Facility, STFC Rutherford Appleton Laboratory, Chilton, Didcot, Oxfordshire, OX11 0QX, United Kingdom*
[6]*University of Warwick, Department of Physics, Coventry, CV4 7AL, United Kingdom*
[7]*Institut Laue-Langevin, CS 20156, 38042 Grenoble Cedex 9, France*
[8]*Laboratory for Muon Spin Spectroscopy, Paul Scherrer Institut, CH-5232 Villigen PSI, Switzerland*

## I. MAGNETIZATION MEASUREMENTS

Figure 1 shows magnetization measurements as a function of temperature in applied magnetic fields corresponding to the LF $\mu^+$SR measurements in Fig. 5 of the main text. For the case of $GaV_4Se_8$ we observe that the peak at the location of the phase transition gradually disappears upon increasing the magnetic field. At 95 mT this peak is relatively wide and the field at which the peak in $GaV_4Se_8$ vanishes suggests that the underlying anisotropy that gives rise to it exists on an energy scale of around 0.1 K. Moreover, we observe a splitting of the curves measured after cooling in zero field (black) and in an applied magnetic field (red) exactly at the temperature where we locate the transition between C and SkL phases.

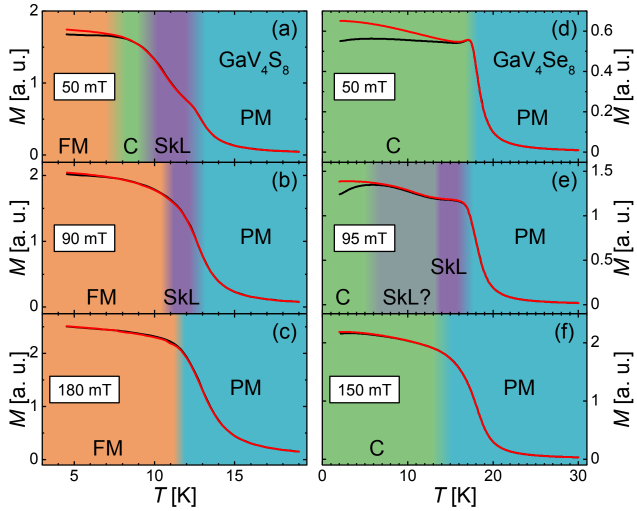


FIG. 1. Magnetization $M$ of $GaV_4S_8$ (left) and $GaV_4Se_8$ (right) as a function of temperature in applied magnetic fields. Measurements were performed both after cooling in zero field (black) and in an applied magnetic field (red). The labeling of the phases is according to $\mu^+$SR data.

## II. IMAGINARY PART OF THE AC SUSCEPTIBILITY

Figure 2 shows the imaginary part $\chi''$ of the AC susceptibility of both $GaV_4S_8$ and $GaV_4Se_8$. Contour lines of the real part are superimposed on the phase diagrams for comparison.

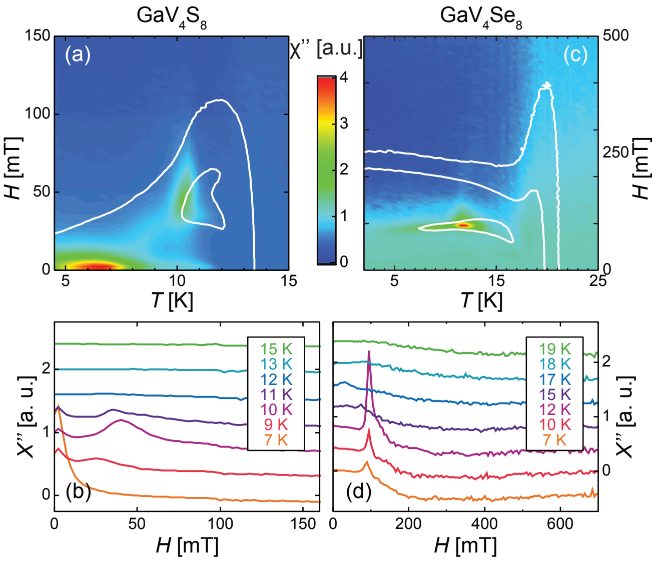


FIG. 2. *Top*: Imaginary part $\chi''$ of the AC susceptibility of (a) $GaV_4S_8$ and (c) $GaV_4Se_8$. White contour lines from the phase diagrams using the real part $\chi'$ of the AC susceptibility. *Bottom*: $\chi''$ as a function of applied field for selected temperatures for (b) $GaV_4S_8$ and (d) $GaV_4Se_8$

## III. TF $\mu^+$SR MEASUREMENTS

Results from fitting TF $\mu^+$SR measurements made on $GaV_4Se_8$ in $\mu_0$H= 50 mT are presented in Fig. 3. FT spectra are shown in Fig. 4(b). As for $GaV_4S_8$ two in-

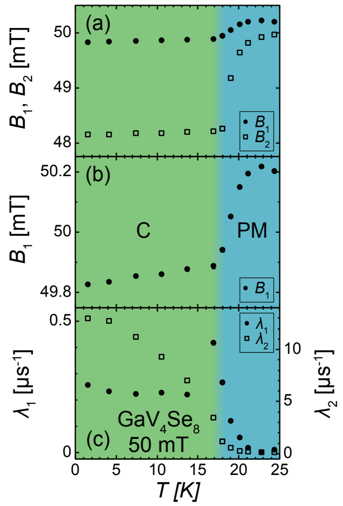


FIG. 3. Fitting of TF data of $GaV_4Se_8$ in an applied field of 50 mT. (a) Internal fields $B_1$ and $B_2$. (b) Enlarged view of $B_1$. (c) Relaxation rates $\lambda_1$ and $\lambda_2$.

ternal fields are observed at all applied magnetic fields, consistent with two inequivalent muon sites. The results can be divided into three different temperature regimes. (I) In the high temperature regime both internal fields are close to each other and the applied magnetic field, and cannot be distinguished in the FT spectra. Both relaxation rates are small. (II) In the intermediate temperature regime both internal fields (especially $B_2$) decrease rapidly and can be resolved in the FT spectra. The relaxation rates increase with decreasing temperature, especially $\lambda_2$, reflected by the $B_2$ peak in the FT spectra broadening out. (III) In the low temperature regime the internal fields still decrease with decreasing temperature, but at a reduced rate. Only $B_1$ can be resolved in the FT spectra as $\lambda_2$ becomes very large. Taking into account the results from LF $\mu^+$SR measurements presented in Fig. 5 of the main text this regime most likely corresponds to the magnetically ordered phase. Note, that in none of the measurements a clear increase in $B_1$ can be observed in any part of the magnetically ordered phase, which was the signature of the SkL for $GaV_4S_8$.

## IV. MUON SITE CALCULATIONS

For our calculations on $GaV_4S_8$, we use a plane wave cutoff energy of 950 eV, resulting in total energies that converge to 0.1 eV per cell and a $4\times4\times2$ Monkhurst-Pack grid[1] for Brillouin zone sampling. We first optimized the ionic positions of the perfect crystal, allowing the ions to move until the energy reaches a convergence threshold; the lattice parameters are held fixed at their experimental values throughout this procedure. We determined muon stopping sites by placing a muon (modelled as an ultra-soft hydrogen pseudopotential) in one of 68 initial positions and then allowing the structure plus implanted muon to relax. For $GaV_4Se_8$, the lattice parameters for the rhombohedral phase have not been previously reported, so we optimize these using DFT (starting from those of $GaV_4S_8$). We used a plane wave cutoff energy of 550 eV and $4 \times 4 \times 2$ Monkhurst-Pack grid for Brillouin zone sampling. Forty structures comprising the unit cell plus an implanted muon (again modelled as an ultra-soft hydrogen pseudopotential) are relaxed to determine the muon stopping sites. Note that DFT claculations have been show to reproduce or predict experimental results accuratly.[2]

We observe that, for both the S and Se members of the series, the muon stopping sites do not correspond to the minima in the electrostatic potential, which themselves occupy interstitial positions around the $GaS_4$ tetrahedra. Disagreement between the muon stopping sites and the electrostatic minima has been found in other systems[3] where strong muon-lattice interactions (in our case the interaction between the muon and S/Se) leads to localization away from the electrostatic minimum.

The results of calculations for $GaV_4Se_8$ are shown in Fig. 5. The sites we find are similar to those calculated for $GaV_4S_8$, with three of the four sites involving the muon sitting close to a Se atom and a site in which the muon sits above a face of a $V_4Se_4$ unit. However, the ordering of sites is different in this case. In particular, the cube face site [site 1] [Fig. 6(1)], which was found to be the highest energy stopping site for $GaV_4S_8$, is the lowest energy site for $GaV_4Se_8$. The sites in which the muon sits near an Se atom can also be compared to analogous sites for $GaV_4S_4$. Site 2 [Fig. 6(2)], which is 0.145 eV higher in energy than the lowest energy site, is similar to site III in $GaV_4S_8$, with the muon bonded to the Se atom at the top of a $GaSe_4$ tetrahedron. Site 3 [Fig. 6(3)] is 0.190 eV higher in energy than the lowest energy site and is similar to site II in $GaV_4S_8$, but with a longer $\mu^+$–Se distance (1.7 Å). Site 4 [Fig. 6(4), 0.381 eV higher in energy than site 1] is similar to site I in $GaV_4S_8$.

We conclude that, although the sites for the two systems are similar owing to their similar structures, the energetic ordering of sites in the two cases is rather different. In particular, the lowest energy site (which we might expect to contribute the greatest fraction of the asymmetry) is different for the two materials despite their structural resemblance. Our resuts show that localization near S seems to be a more important factor than localization near Se. This likely due to the higher electronegativity of S.

These calculations were motivated by the unusual increase of the total local magnetic fields $B_1$ with temperature in our ZF $\mu^+$SR measurements on $GaV_4S_4$. We therefore suggested that the field at the muon stopping sites behaves in a different way to the bulk magnetization. A temperature dependent hyperfine contribution at the muon site could be responsible for this. This is supported by the observation of a large Knight shift in the TF $\mu^+$SR spectra for $GaV_4S_8$, indicating a significant hyperfine coupling at the muon site. We find that

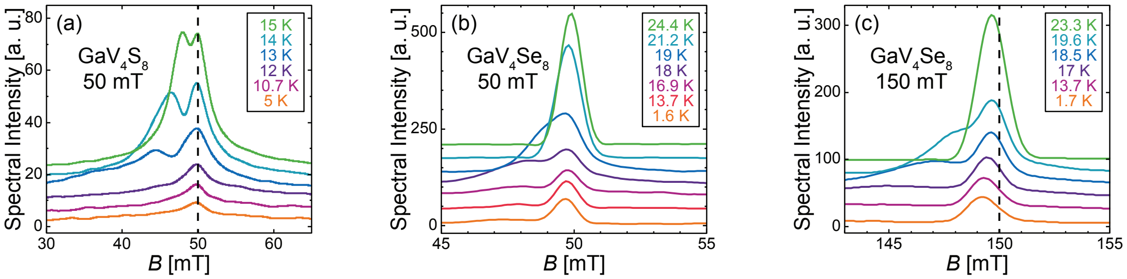


FIG. 4. Evolution of the internal magnetic field distribution with $T$ in (a) $GaV_4S_8$ in a TF of 50 mT, (b) $GaV_4Se_8$ in a TF of 50 mT, and (c) $GaV_4Se_8$ in a TF of 150 mT. Curves have been offset for clarity.

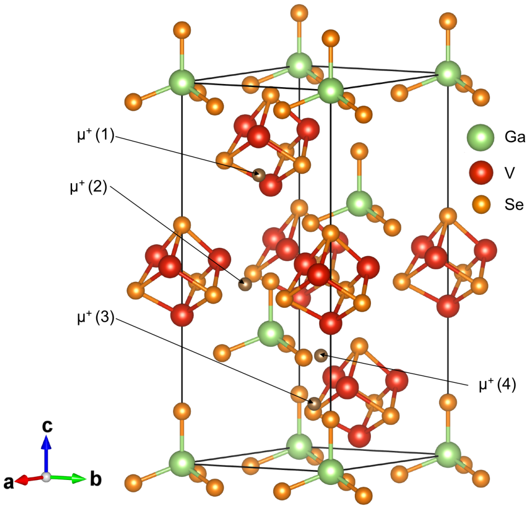


FIG. 5. The four distinct muon stopping sites determined for $GaV_4Se_8$. Sites are numbered in order of increasing energy.

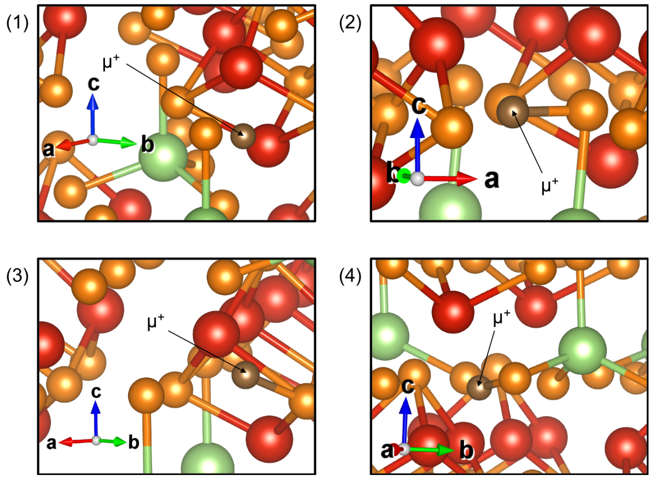


FIG. 6. The local geometry around the muon for each of the four classes of muon stopping site.

for the lowest energy sites in each of the compounds the muon attract significant *electronic* density in its vicinity, forming a state that has close to zero charge. We refrain from calling this state muonium due to the fact that the *spin* density associated with the muon is very small in both cases (whereas muonium refers to the bound state of $\mu^+$ and an S=1/2 electron). These results leave open the possibility of a significant hyperfine contribution to the local magnetic field at the muon site, though the smallness of the spin density prevents us from concluding strongly in favour of its existence. We do not observe any significant structural distortions induced by the muon, which could affect the local magnetic properties. We attempted to investigate the effect of the implanted muon on the spin configuration, but found that DFT calculations would fall into one of many vastly different magnetic states that are close in energy, which made it difficult to draw robust conclusions about the influence of the muon.

Zhang et al.[4] reported a failure of DFT in correctly predicting a band gap in $GaV_4S_8$. In our PBE calculations we find that the Fermi energy crosses bands for one of the spin channels, making the material a semi-metal. This means that the muon sites detailed above have been calculated on a system with different electronic properties to those observed experimentally. To address this deficiency we have carried out DFT+U calculations, taking the calculated muon stopping sites as our starting point. Using the LDA exchange-correlation functional and applying a Hubbard $U$ of 2.5 eV to the V $d$-orbitals we allow each of the sites to further relax. We find that the muon sites are unchanged by this procedure. Surprisingly, PBE+U calculations on $GaV_4S_8$ fail to produce a band gap even for $U$ values up to 4.5 eV. However, PBE+U calculations with $U$=3.5 eV were found to result in the same sites determind using the altenative exchange-correlation functionals. We therefore conclude that the muon stopping sites in this system are not sensitive to the precise form of the exchange-correlation functional used and that calculations at the previous level of complexity (GGA) are sufficient for accurately determining muon stopping sites, despite their failure to properly reproduce all of the material properties.

To help assign each of the calculated muon sites to the sites observed in our $\mu^+$SR measurement we have carried out dipolar field calculations for $GaV_4S_8$. We take a magnetic moment of 1.73 $\mu_B$ per formula unit, corresponding to one unpaired electron $V_4$ cluster, which has

been found to be consistent with values obtained from susceptibilty measurements.[5] We take the moment to be localized on the apical V atom and aligned along [111], the magnetic easy axis in this material.[6] The dipolar field experienced by a muon at position $\mathbf{r}_\mu$ due to the magnetically ordered structure is given by

$$\mathbf{B}_{\rm dipole}(\mathbf{r}_\mu) = \sum_i \frac{\mu_0}{4\pi r^3}\left[3(\boldsymbol{\mu}_i \cdot \hat{\mathbf{r}})\hat{\mathbf{r}} - \boldsymbol{\mu}_i\right] \qquad (1)$$

where $\mu_0$ is the permeability of free space and $\mathbf{r} = \mathbf{r}_\mu - \mathbf{r}_i$ is the position of the muon relative to ion $i$ with magnetic moment $\boldsymbol{\mu}_i$. Calculating the dipolar field associated with each of the muon stopping sites I–IV we find $B = 49, 85, 52, 39$ mT respectively. Because the spin structure is ferromagnetic we need to also consider the effect of the Lorentz and demagnetizing fields. These contributions are proportional to the net magnetization of the sample and are therefore independent of the muon stopping site. These terms act to reduce the magnetic field experienced by the muon at each of the stopping sites. Assuming that the two precession frequencies observed in the ZF data corresond to the two lowest energy sites here we assign $B_1$ to Site II and $B_2$ to Site I. Assuming $B_{\rm L} + B_{\rm d} = -37$ mT, the total field at each site (neglecting any hyperfine contribution) $B_{1,\rm calc} = 48$ mT and $B_{2,\rm calc} = 12$ mT have magnitudes in the ratio 4:1. These values are slightly higher than those obtained in the experimental data, but seem quite plausible. There is of course also the possibility of significant different hyperfine contributions at the two muon stopping sites, as suggested by the TF $\mu^+$SR data. We must also consider that the approximation of the moments being located at a single point is a crude one, particularly given that the fields at each of the muon sites is likely to be highly sensitive to the distribution of spin around the nearest $V_4S_4$ unit. Taking the above considerations into account, these calculations show that the calculated muon sites may be plausibly mapped to those observed experimentally, based on the magnitudes of the fields experienced by the muon at each of these sites.


[1] H. J. Monkhorst and J. D. Pack, Phys. Rev. B **13**, 5188 (1976).

[2] K. Lejaeghere, G. Bihlmayer, T. Björkman, P. Blaha, S. Blügel, V. Blum, D. Caliste, I. E. Castelli, S. J. Clark, A. D. Corso, S. d. Gironcoli, T. Deutsch, J. K. Dewhurst, I. D. Marco, C. Draxl, M. Dułak, O. Eriksson, J. A. Flores-Livas, K. F. Garrity, L. Genovese, P. Giannozzi, M. Giantomassi, S. Goedecker, X. Gonze, O. Grånäs, E. K. U. Gross, A. Gulans, F. Gygi, D. R. Hamann, P. J. Hasnip, N. a. W. Holzwarth, D. Iuşan, D. B. Jochym, F. Jollet, D. Jones, G. Kresse, K. Koepernik, E. Küçükbenli, Y. O. Kvashnin, I. L. M. Locht, S. Lubeck, M. Marsman, N. Marzari, U. Nitzsche, L. Nordström, T. Ozaki, L. Paulatto, C. J. Pickard, W. Poelmans, M. I. J. Probert, K. Refson, M. Richter, G.-M. Rignanese, S. Saha, M. Scheffler, M. Schlipf, K. Schwarz, S. Sharma, F. Tavazza, P. Thunström, A. Tkatchenko, M. Torrent, D. Vanderbilt, M. J. v. Setten, V. V. Speybroeck, J. M. Wills, J. R. Yates, G.-X. Zhang, and S. Cottenier, Science **351**, aad3000 (2016).

[3] J. S. Möller, D. Ceresoli, T. Lancaster, N. Marzari, and S. J. Blundell, Phys. Rev. B **87**, 121108 (2013).

[4] J. T. Zhang, J. L. Wang, X. Q. Yang, W. S. Xia, X. M. Lu, and J. S. Zhu, Phys. Rev. B **95**, 085136 (2017).

[5] D. Johrendt, Z. Anorg. Allg. Chem. **624**, 952 (1998).

[6] I. Kézsmárki, S. Bordács, P. Milde, E. Neuber, L. M. Eng, J. S. White, H. M. Rønnow, C. D. Dewhurst, M. Mochizuki, K. Yanai, H. Nakamura, D. Ehlers, V. Tsurkan, and A. Loidl, Nat. Mater. **14**, 1116 (2015).
